# Supplementary material for: Modeling the Impact of Network Connectivity on Consensus Security of Proof-of-Work Blockchain
Source: arXiv:2002.08912 source file (2020-08-31)
Supplement: Supplementary file 1 [file appendix.tex]

\section{Calculating the Winning Probability}

\subsection{Reduction to Regular Graph}
\label{appendix:reduction}
